# Supplementary material for: CausCF: Causal Collaborative Filtering for RecommendationEffect Estimation
Source: arXiv:2105.13881 source file (2021-05-28)
Supplement: Supplementary file 1 [file appendix.tex]

\section{Experiments on Semi-synthetic Dataset.}
